# Supplementary material for: Optimizing User Interface Layouts via Gradient Descent
Source: arXiv:2002.10702 ancillary file (2020-02-25)
Supplement: Supplementary file 1 [file additional_initial_and_optimized_layouts.pdf]

This supplementary document includes additional optimization results for both UIs. The task performance improvements are all predicted by the model.

**Photo Editing UI:**

The following layouts were optimized using strict constraints, as described in the main text. The constraints include large minimum size limits for all UI elements, identical sizes between the undo and upload icons, and grouping the sticker button with the stickers.  All these layouts are initially bad.

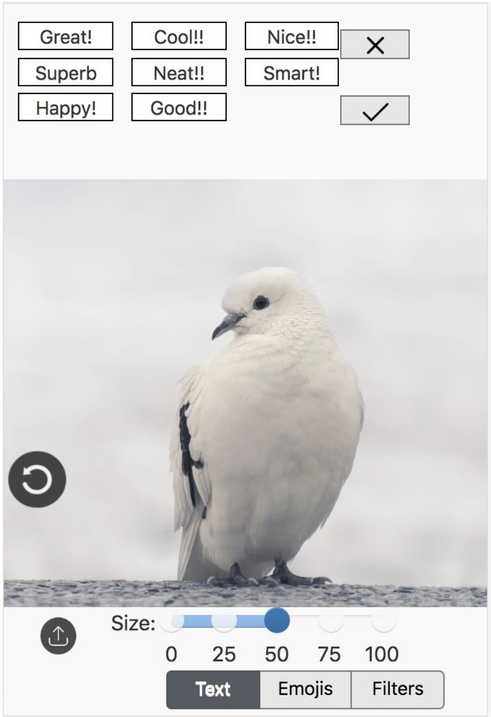


Initial

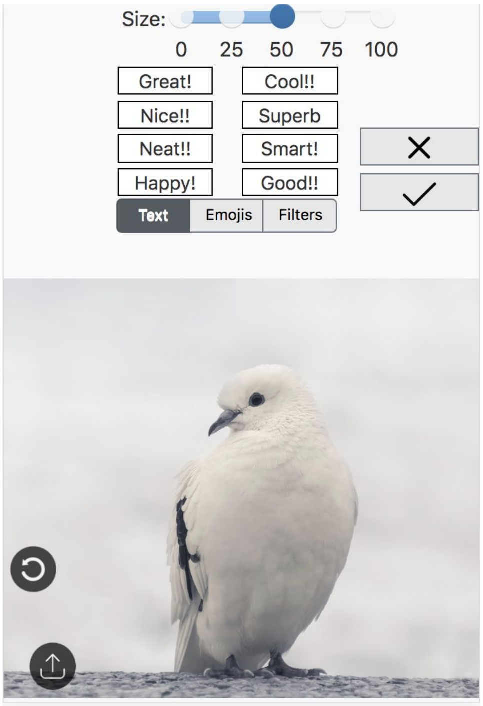


Optimized: (17.8% improvement)

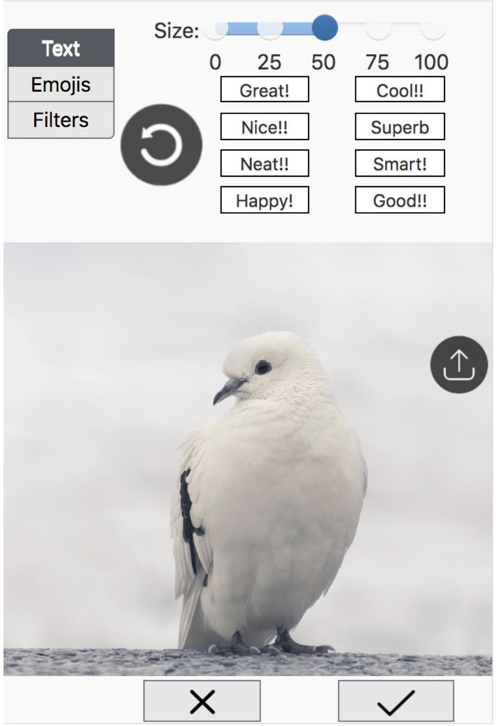


Initial

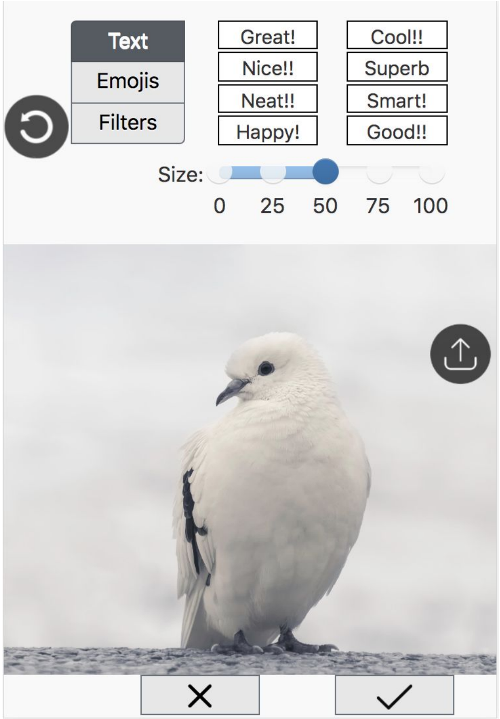


Optimized (3.2% improvement)

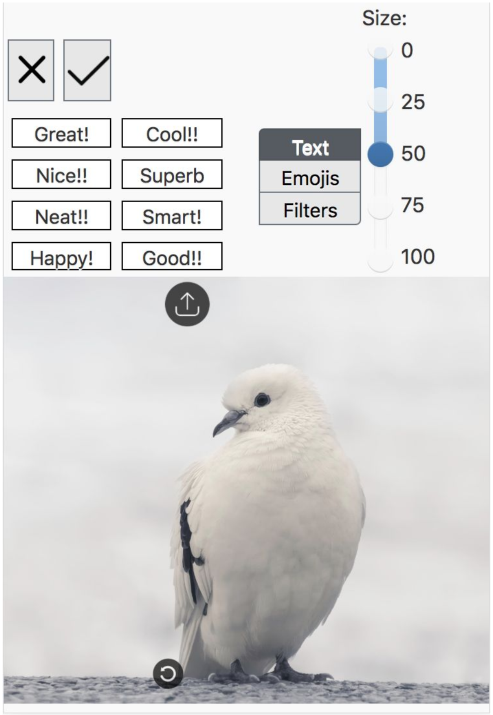


Initial

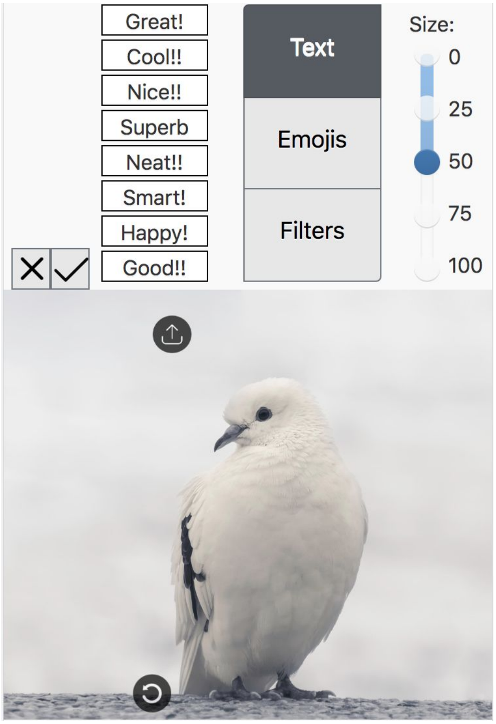


Optimized (3.3% improvement)

**Recipe Planning UI**

The following layouts were optimized using only lenient minimum size penalties as described in the main text. The algorithm's output layout was then tweaked slightly for sizing and alignment.

Initially Bad Layout:

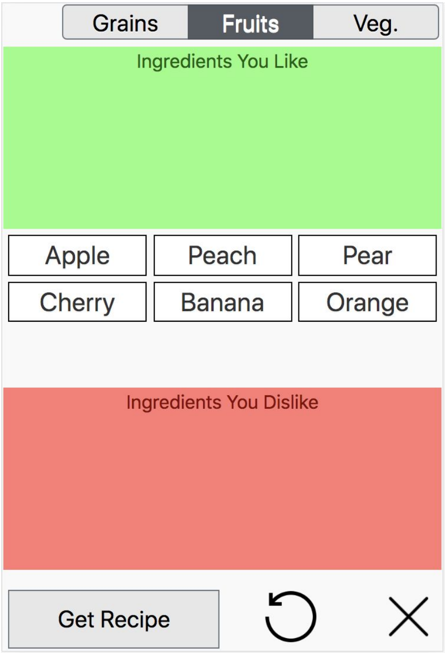


Initial

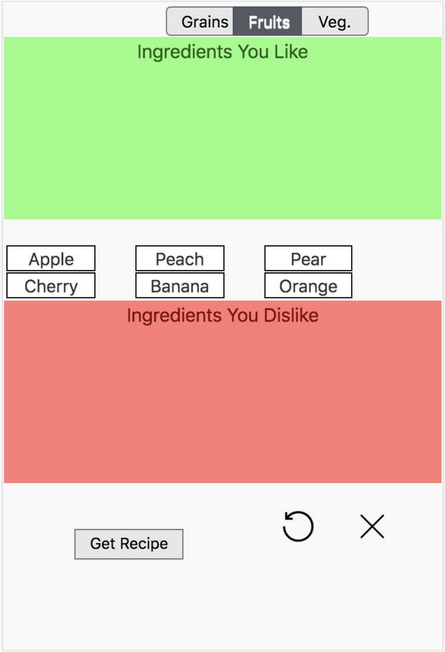


Optimized + tweaking (2.9% improvement)

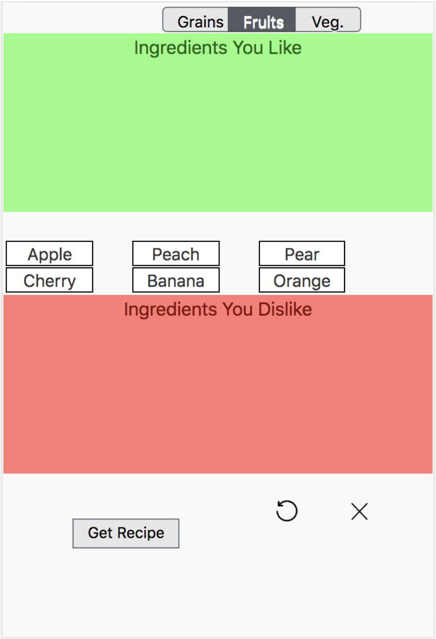


Optimized: (3.6% improvement)

Initially Good Layout:

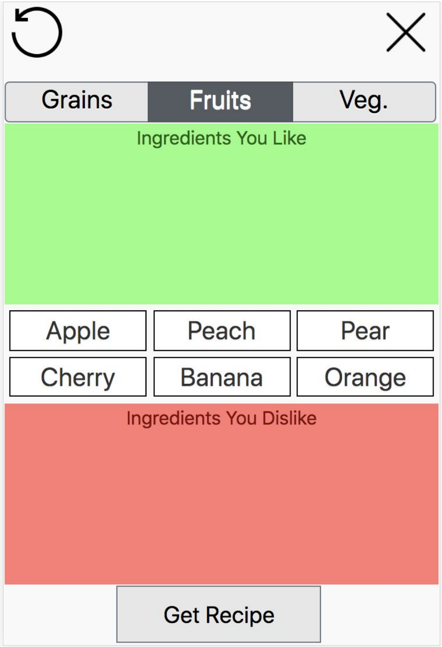


Initial

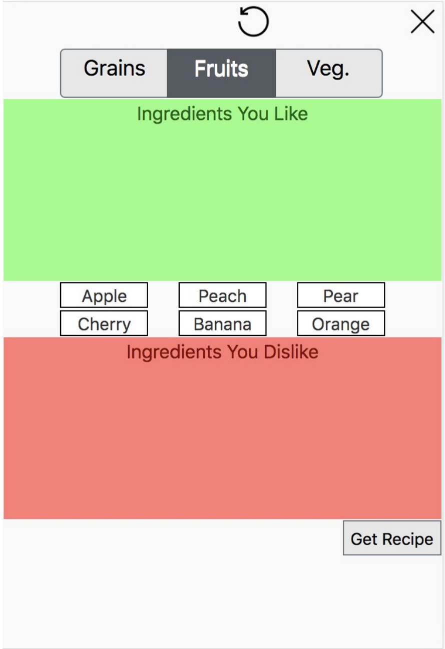


Optimized + tweaking (5.3% improvement)

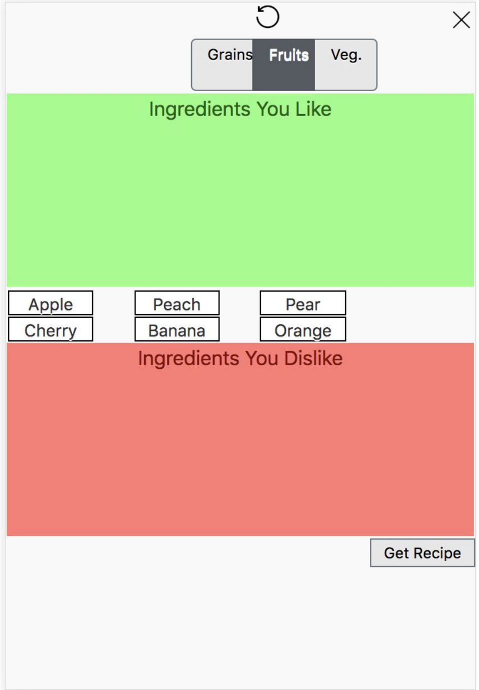


Optimized (7.2% improvement)
