# Supplementary material for: Optimizing User Interface Layouts via Gradient Descent
Source: arXiv:2002.10702 ancillary file (2020-02-25)
Supplement: Supplementary file 2 [file data_collection_app_and_optimization.pdf]

# Supplementary Materials: Data Collection App and Optimization Details

## DOCUMENT DESCRIPTION

This supplementary document contains details of the data collection app and the optimization algorithm.

## DATA COLLECTION APP

This section contains details of our data collection app. Following the data collection app from Deep Menu, the task sequence is presented to the mTurk worker in a the following manner: the worker first sees the instructions for the task, and when users are ready to complete the task, they tap the start button, where they are taken to the UI to complete the task. Figure 1 illustrates this flow. We also show an image of the target for task instructions where the target is an icon or an image (see Figure 1), since we are using this model to optimize for layout and not icon nor image choice. Showing workers what the target looks like prevents extra time on the task due to confusion caused by factors such as poor icon choice or ambiguous descriptions of the target in the instructions. We record mistakes in the task sequence; if workers made a mistake on a task, they are asked to redo the task it until they have completed it correctly. Our app also kept track of the changes users have made to the current photo as they work through the task sequence. If the worker incorrectly tapped the save or cancel button, they were taken back to the first task for the current photo and would have to continue from there. These mistake penalties are to simulate realistic consequences of making mistakes in the interface, to capture more realistic task performance times as users take more care to avoid making mistakes while completing tasks. To incentivize workers to be as accurate as possible when completing the task sequence, they are given a bonus at the end based on their accuracy in completing the tasks. In case users forget the task's instructions, they can see the task's instructions again. This is to prevent errors or extra time users may spend trying to recall the instructions. To encourage workers to read the task's instructions carefully the first time, viewing the task's instructions more than once decreases their bonus. Finally, since our task sequence is quite long, workers were reminded to take a break every 50 tasks to prevent fatigue. They also had the option to take a break when they are at any task's instructions page. We impose a 5-minute time limit on the UI page to prevent workers from taking breaks when they are supposed to be completing the task.

ACM ISBN 978-1-4503-2138-9.
DOI: 10.1145/1235

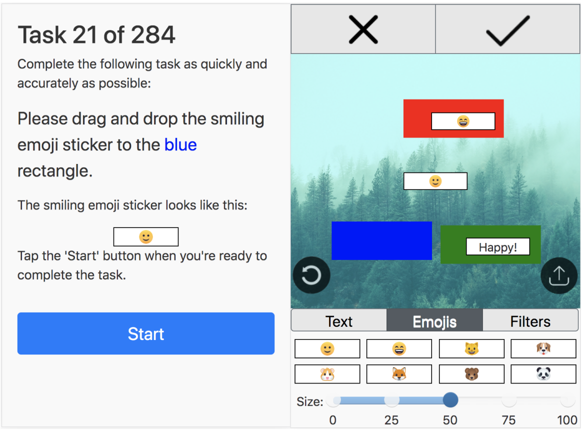


**Figure 1. The data collection app, with the task instructions page (page) and the UI page (right). When workers are ready to complete the task after reading the instructions, they tap on the "Start" button and are taken to the UI to complete the task.**

To ensure that each worker sees the expected rendition of their assigned layout, workers are required to complete the task sequence on an IPhone 6, 6s, or 7, which all have the same screen size. Furthermore, workers must complete the task sequence in portrait mode. If their phone is detected to be in landscape mode, they are unable to continue until they have switched the phone back to portrait mode. These phone and orientation constraints were also enforced in Deep Menu's data collection app. Our data collection app also disabled zooming and scrolling when the user is on the page with the photo editing interface.

### Data Collection Methodology

As mentioned in the main text, the legal department at our institution reviewed the project proposal and authorized the data collection protocol prior to initiation of the study. We provided all prospective participants with a detailed description of the data collection process in the consent form that was displayed and acknowledged by the participants prior to their acceptance in the study. Participants could opt-out (not continue with the study) if they were uncomfortable with the scope of the consent, or the elements of the study at any time during the course of their participation..

## OPTIMIZATION

This section discusses the the penalty functions we used, and provides other details of our optimization algorithm. As described in the main text, we will be optimizing the following

objective function $F$ for layout $l$:

$$
\begin{aligned}
F(l) = {} & task\_seq\_perf(l) \\
& + (penalty\_constant)(overlap\_penalty(l)) \\
& + (penalty\_constant)(boundary\_penalty(l)) \\
& + (penalty\_constant)(additional\_penalties(l))
\end{aligned} \tag{1}
$$

Where $task\_seq\_perf$ is the sum of the predicted task performance of all tasks in the sequence, $overlap\_penalty$ is a differentiable function that is positive if there are overlapping UI elements in layout $l$ and is 0 otherwise. Likewise, $boundary\_penalty$ is a differentiable function that is positive only if any element in $l$ exceeds the boundary of the user interface. $additional\_penalties$ refers to penalty functions of additional constraints the designer hopes to enforce, e.g. ensuring two particular elements are aligned. $penalty\_constant$ and is a constant that adds a high value to the objective function if its corresponding penalty function is positive.

### *Penalty Functions: Boundary and Overlap*

As mentioned earlier, the spatial aspects of each UI element are represented in pixels. The UI can be represented as a 2-dimensional coordinate system bounded by the dimensions of the phone screen. The top left corner defined as $(0px, 0px)$ and the bottom right corner is $(screen\_widthpx, screen\_heightpx)$. Hence, the boundary penalty $bp$ function for UI element $u$ is defined as the sum of the

$$
\begin{aligned}
bp(u) = {} & ReLU(-(x_u - width_u/2)) \\
& + ReLU(x_u + width_u/2 - screen\_width) \\
& + ReLU(-(y_u - height_u/2)) \\
& + ReLU(y_u + height_u/2 - screen\_height)
\end{aligned} \tag{2}
$$

$x_u$ represents the $x$ feature of Equation 1 in the main text and is the horizontal location of center of the element $u$. Hence, $x_u - width_u/2$ is the horizontal location of the left edge of $u$ or it's rectangular boundary. For grouped elements, $x_u$ and $width_u$ are replaced by $container\_x_u$ and $container\_width_u$, respectively. If $x_u - width_u/2 < 0$, then the element has exceeded the left boundary of the UI screen, which results in positive values for $-(x_u - width_u/2)$ and $ReLU(-(x_u - width_u/2))$. Likewise, if $x_u + width_u/2 > screen\_width$, then $u$ has exceeded the right boundary of the UI, leading to a positive value for $ReLU(x_u + width_u/2 - screen\_width)$. The boundary penalty functions for $y_u$ and $height_u$ follow the same definition. Thus, if element $u$ exceeds any edge of the UI boundary $bp(u)$ becomes positive, adding a penalty to the objective function. The $boundary\_penalty(l)$ term from Equation 1 is defined as the sum of the $bp$ penalty function for all elements in the interface. Hence, $boundary\_penalty(l)$ would be activated when any UI element in layout $l$ exceeds the interface's boundary.

For two elements in a UI to overlap, the horizontal distance between their centers must be less than half the sum of their respective widths and the vertical distance must be less than half the sum of their respective heights, as illustrated in Figure 2. Any other conditions will not lead to an overlap. We use the following overlap penalty function $op$ to detect overlap

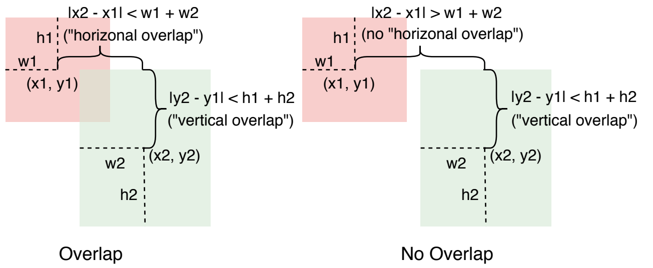


**Figure 2. This figure shows that there must be both horizontal and vertical overlap between two elements for them to overlap. There is no overlap between the two elements under any other conditions.**

between two elements $u_1$ and $u_2$

$$
\begin{aligned}
& op(u_1, u_2) = \\
& ReLU(((width_{u,1} + width_{u,2})/2)^2 - (x_{u,1} - x_{u,2})^2) \\
& \times ReLU(((height_{u,1} + height_{u,2})/2)^2 - (y_{u,1} - y_{u,2})^2)
\end{aligned} \tag{3}
$$

The horizontal distance between $u_1$ and $u_2$ is represented as $abs(x_{u,1} - x_{u,2})$. The horizontal distance being less than half the sum of their widths (i.e. "horizontal overlap") is represented by the following equation:

$$abs(x_{u,1} - x_{u,2}) < (width_{u,1} + width_{u,2})/2 \tag{4}$$

Squaring both sides eliminates the undifferentiable absolute value function. Rearranging the terms and multiplying both sides by $-1$ yields

$$((width_{u,1} + width_{u,2})/2)^2 - (x_{u,1} - x_{u,2})^2 > 0 \tag{5}$$

The left hand side of Equation 5 is equal to the argument to the first $ReLU$ function of Equation 3. Hence, if there is a "horizontal overlap", Equation 4 holds, which leads to the first $ReLU$ function of the product in Equation 3 to be positive. Since both a "horizontal overlap" and a "vertical overlap" must occur for $u_1$ and $u_2$ to actually overlap, the two $ReLU$ functions are multiplied in Equation 3, so that $op(u_1, u_2)$ is positive if both $ReLU$ functions in the product are positive. If either $ReLU$ function is 0, then there is no overlap between $u_1$ and $u_2$ and $op(u_1, u_2)$ becomes 0. The $overlap\_penalty(l)$ term from Equation 1 is hence defined as

$$overlap\_penalty(l) = \sum_{u_1, u_2 \in l, u_1 \neq u_2} op(u_1, u_2) \tag{6}$$

Thus, $overlap\_penalty(l)$ is greater than 0 if any two elements in layout $l$ overlap.

### *Additional Penalty Functions*

In addition to the necessary overlap and boundary penalty functions, designers can add more constraints to improve the output of the optimization. For instance, penalty functions can be enforced for two UI elements $u_1$ and $u_2$ to have the same size by the following equation:

$$
\begin{aligned}
& identical\_size(u_1, u_2) = \\
& ReLU((height_u, 1 - height_u, 2)^2) \\
& + ReLU((width_u, 1 - width_u, 2)^2)
\end{aligned} \tag{7}
$$

Where $identical\_size(u_1, u_2)$ is greater than 0 if $u_1$ and $u_2$ differ in height and width. Furthermore, a minimum size penalty can be added to keep the *height* or *width* of element $u$ to be greater than a lower bound $C$. This can be enforced by the function

$$min\_size(u_1) = ReLU(C - width_u, 1) \quad (8)$$

Finally, if a designer wants to group two elements together, such as the sticker button group (Section D of Figure 3) with the stickers (Section E), they can introduce a penalty function to ensure the two elements are in close proximity, align them horizontally or vertically, and ensure they have the same size dimension along their bordering sides (e.g. the sticker button and stickers in Figure 3) should have the same *width*s). This *group* penalty function for sticker button group $b$ and stickers $s$ is expressed as

$$\begin{aligned} group(s,b) &= ReLU((width_s - width_b)^2) \\ &+ ReLU((x_s - x_b)^2) \\ &+ ReLU((y_s - y_b)^2 - ((height_s + height_b)/2)^2 - c) \end{aligned} \quad (9)$$

$ReLU((width_s - width_b)^2)$ ensures that the sticker button and sticker group have the same width, $ReLU((x_s - x_b)^2)$ ensures that the two elements are aligned horizontally, and $ReLU((y_s - y_b)^2 - ((height_s + height_b)/2)^2 - c)$ ensures that they are in close vertical proximity. The $(y_s - y_b)^2 - ((height_s + height_b)/2)^2$ term pulls the two elements together vertically, since the penalty function increases with their vertical distance. The term $c$ is a positive constant and is is added to enforce some vertical gap between the sticker button and sticker group. In sum, penalty functions can be added to ensure any desired characteristics in the optimized layout.

### Swapping Locations of UI Elements

At each optimization step, if two UI elements $u_1$ and $u_2$ overlap and their gradients $\frac{\partial F'}{\partial y_{u,1}}$ and $\frac{\partial F'}{\partial y_{u,2}}$ satisfy one of the following three conditions, then $u_1$ and $u_2$ are swapped vertically. Assume $u_1$ is located above $u_2$, and a vertical swap will move $u_2$ above $u_1$ if one of the following conditions hold:

1. $\frac{\partial F'}{\partial y_{u,1}} > 0$ and $\frac{\partial F'}{\partial y_{u,2}} < 0$
2. $\frac{\partial F'}{\partial y_{u,1}} - 2\frac{\partial F'}{\partial y_{u,2}} > 0$
3. $\frac{\partial F'}{\partial y_{u,2}} - 2\frac{\partial F'}{\partial y_{u,1}} < 0$

Note, $F'$ refers to the objective function from Equation 1 without the overlap penalty function. Condition 1 is when the top element $u_1$ wants to move down while the bottom element $u_2$ wants to move up, so a vertical swap would likely lead to a decrease in the objective function. Condition 2 is when $u_1$ has strong downward $y$ gradient with magnitude twice the downward $y$ gradient of $u_2$, which means a vertical swap to move $u_1$ below $u_2$ may decrease the objective function. Likewise, Condition 3 shows a significantly stronger upward $y$ gradient for $u_2$. A vertical swap of $u_1$ and $u_2$ is a vertical reflection of $u_1$ and $u_2$ along the x-axis located along the vertical midpoint of those two elements. Since $u_1$ and $u_2$ overlap, after the vertical reflection, both elements are pushed away from each other

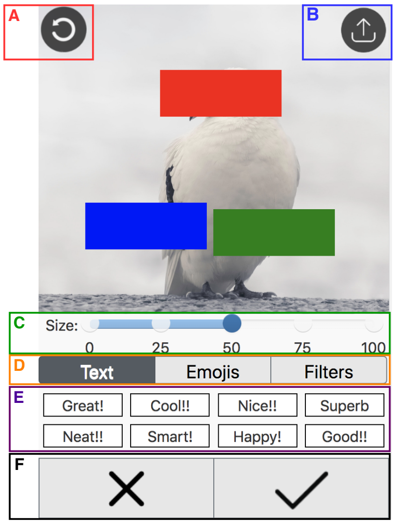


**Figure 3. The photo editing UI with all the UI elements labelled. A is undo icon, B is the upload icon, C is the slider, D is the button group that controls which set of stickers are displayed, E is the set of stickers (icon group type), and F is the button group with the save (checkmark) and cancel ("X") buttons. The colored rectangles in the photo are not part of the UI; they are the drop targets for drag and drop tasks (Task Type 4).**

vertically to eliminate the overlap. Horizontal swaps follow a similar set of conditions and swap procedures. If conditions are met for both a horizontal and vertical swap, the swap with the larger decrease in the objective function is performed.

### Maintaining Invariants in Element Types

For certain UI element types, some constraints must be made during the updates. For instance, icons must maintain their width to height aspect ratio during the updates. To retain the aspect ratio, either the *height* or *width* gradient (the larger of the two) is used to update the corresponding feature, and the other feature is updated with the same gradient scaled by the aspect ratio. In addition, for icon groups to maintain their grid structure (see Figure 3 Section E for an example of an icon group), after the size updates have been made both to the icons and the container, the locations of the icons within the container are recomputed to retain the grid structure of evenly spaced icons.
